# Supplementary material for: SHACL Constraints with Inference Rules
Source: arXiv:1911.00598 source file (2019-11-01)
Supplement: Supplementary file 1 [file ISWC-Appendix-Only.tex]

\documentclass[runningheads]{llncs}

%\pdfpagewidth=8.5in
%\pdfpageheight=11in

\usepackage{times}
\usepackage{soul}
\usepackage{url}
\usepackage[hidelinks]{hyperref}
\usepackage[utf8]{inputenc}
\usepackage[small]{caption}
\usepackage{graphicx}
\usepackage{amsmath}
\usepackage{booktabs}
\usepackage{algorithm}
\usepackage{arevmath}     % For math symbols
\usepackage[noend]{algpseudocode}
\usepackage{listings,multicol}
\urlstyle{same}
\usepackage{multicol}
\usepackage{longtable}

\usepackage[caption=false]{subfig}

\usepackage{oz}
\usepackage{makeidx}
\usepackage{listings}
\usepackage{amsfonts}
\usepackage{relsize}
\usepackage{urwchancal}
\usepackage{stmaryrd}
\usepackage{ dsfont }
\usepackage{placeins}
\usepackage{longtable}
\usepackage{standalone}

\usepackage{float}
\newfloat{algorithm}{t}{lop}

%\usepackage[colorinlistoftodos]{todonotes}
%\newtheorem{theorem}{Theorem}[section]
%\newtheorem{lemma}[theorem]{Lemma}
%\newtheorem{definition}{Definition}[section]

%\newtheorem*{theorem*}{Theorem}

% Score Proof Notation
% First direction
 %               t_o         -->     t^S
 %              t_o^c       -->     t^I
 %   t_o'        -->     t_{\score}
 %             t_a         -->     t_A^I
 %            t_a^o       -->     t_A^S
%   t_s         -->     t_A^{\mathds{S}}
 % t_A'        -->     t_A^{\prime}}
%t_A^{o'}    -->     t_A^{S\prime}}
% Second direction
 %               t_c         -->     t_C
 %               t_A
 %t_A
 %t_q

\usepackage[misc,geometry]{ifsym} 

%\nocopyright

\lstset{
  basicstyle=\ttfamily,
  mathescape
}

\hypersetup{
     colorlinks = true,
     linkcolor = blue,
     anchorcolor = blue,
     citecolor = blue,
     filecolor = blue,
     urlcolor = blue
     }

\let\oldmaketitle\maketitle
\renewcommand{\maketitle}{\oldmaketitle\setcounter{footnote}{0}}

\begin{document}

\appendix
\input{appendices_inner_content.tex}

\end{document}
